# Supplementary material for: Robust line-of-sight pointing control on-board a stratospheric balloon-borne platform
Source: arXiv:2112.10458 source file (2021-12-20)
Supplement: Supplementary file 1 [file 6_appendix.tex]

% \section*{Appendix}
